# Supplementary material for: Electrokinetic Current Driven by a Viscosity Gradient
Source: arXiv:1807.09106 source file (2018-11-16)
Supplement: Supplementary file 1 [file supplemental.pdf]

## SUPPLEMENTAL

### Viscosity profile inside the nanofluidic mixing channel

The theoretical model of viscophoresis presented in the main text uses the viscosity profile inside the nanofluidic mixing channel, $\eta(x)$, where $x$ is the distance from the channel's left end. We calculated $\eta(x)$ based on two assumptions: First, we presume that the viscosity of a mixture of two liquids obeys

$$\eta(\phi) = \eta_f^{1-\phi}\eta_g^{\phi}, \tag{1}$$

where $\phi$ is the volume fraction of the liquid with viscosity $\eta_g$, and $\eta_f$ the viscosity of the other liquid. Equation 1 is a common approximation that is well supported experimentally and theoretically [2, 5]; it also describes the measured dependence of $\eta$ on $\phi$ in our experiments well, as seen in Figure S1. In order to apply eq. 1 to our experiments, $\eta_g$ corresponds to the viscosity of a 50 % water and 50 % glycerol mixture, while $\eta_f$ corresponds to the viscosity of a 50 % water and 50 % formamide mixture.

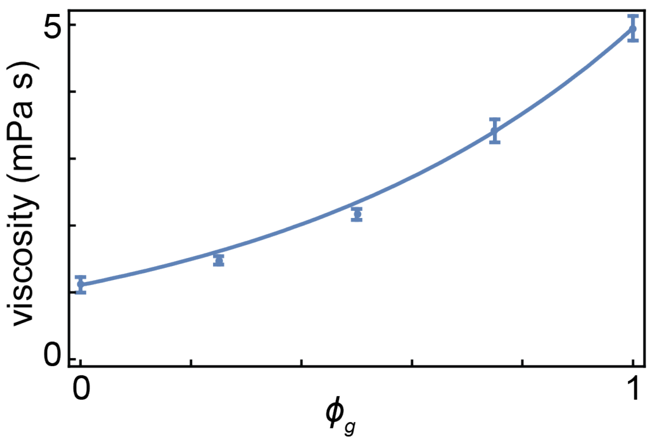


FIG. 1. Dependence of the viscosity of a mixture of two liquids on the volume fraction of the higher-viscosity component. Symbols show measured viscosity of a mixture containing 50 % water, $\phi_g \times$ 50 % glycerol, and $(1-\phi_g)\times 50$ % formamide. The solid line shows eq. 1, where $\eta_f = 1.11\,\mathrm{mPa\,s}$ and $\eta_g = 5.96\,\mathrm{mPa\,s}$.

Second, we assume that as the molecules that comprise the liquids intermix, they execute Brownian motions with an isothermal integration rule, i.e. they obey the same equations of motion as the counterions whose currents we have measured. It is well known that isothermal integration rule also corresponds to the "Fick" generalization of the diffusion equation [4]

$$\frac{d\phi_i}{dt} = \frac{d}{dx}D_i(x)\frac{d\phi_i}{dx}, \tag{2}$$

where $\phi_i$ is the volume fraction of diffusing species $i$, and $D_i(x)$ is its local diffusion coefficient.

Combining equations 1 and 2, we find that in the steady state $\frac{1}{\eta^2}\frac{d\eta}{dx}$ is constant inside the channel. Integrating and applying the boundary conditions $\eta = \eta_L$ at $x = 0$ and $\eta = \eta_R$ at $x = L$ leads to the theoretical viscosity profile inside the mixing channel

$$\eta(x) = \left[\frac{1}{\eta_L} - \frac{x}{L}\left(\frac{1}{\eta_L} - \frac{1}{\eta_R}\right)\right]^{-1}. \tag{3}$$

### Viscophoretic drift speed and counterion current inside the mixing channel

The isothermal integration rule for stochastic processes leads to a very simple equation for a Brownian particle's drift speed in the presence of multiplicative noise [6]

$$\langle \dot{x} \rangle = \frac{dD(x)}{dx}. \tag{4}$$

We combine eq. 4 with the diffusivity profile, $D(x)$, which we obtain from eq. 3 and the Stokes-Einstein relation $D = \frac{k_BT}{6\pi r}\frac{1}{\eta}$ for a spherical particle of hydrodynamic radius $r$, to find the viscophoretic drift speed of the counterions

$$\langle \dot{x}(t) \rangle = -\frac{k_BT}{6\pi rL}\left(\frac{1}{\eta_L} - \frac{1}{\eta_R}\right). \tag{5}$$

We multiply the drift speed in eq. 5 by the total counterion charge density on the top and bottom surfaces of the nanofluidic slit, $2\sigma$, and by the width of the slit, $w$, to find the ionic current associated with the viscophoretic drift of counterions

$$I_v = -\frac{k_BT\sigma w}{3\pi rL}\left(\frac{1}{\eta_L} - \frac{1}{\eta_R}\right). \tag{6}$$

### Width of the boundary layers at the ends of the mixing channel

We used flows in the microchannels of our fluidic chips to refresh the solutions at either end of the mixing channel and maintain a controlled viscosity gradient. Nevertheless, the inter-mixing of the liquids in the channel and in the microchannels creates diffuse transition regions that increase the effective length of the mixing channel. This effect can influence the magnitude of the viscosity gradient. In this section, we theoretically calculate the width of the diffuse boundary layers at the ends of the mixing channel.

We take the flows in the microchannels to be in the positive $y$ direction with constant and uniform speed $u$. Diffusion acts to transport molecules in the $x$ direction. The interface between a microchannel and the mixing channel is illustrated in figure 2. A molecule of the fluid with diffusion coefficient $D$ will diffuse a characteristic distance $\sqrt{Dt}$ in a time $t$. The time it takes fluid flowing in the microchannel to traverse the width $w$ of the mixing channels is $t = w/u$. Therefore, as fluid in a microchannel flows past the end of the mixing channel, diffusion creates a boundary layer that grows in width as

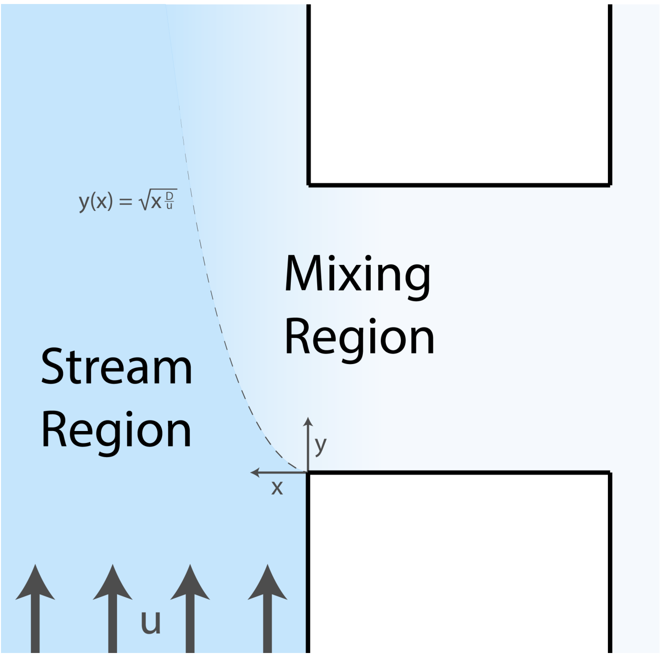


FIG. 2. Sketch of the mixing region extending into a microchannel.

$\sqrt{\Delta y}$ to a maximum value of $\sqrt{Dw/u}$ at the far edge of the mixing channel. The mean width of the boundary layer over the width of the mixing channel is

$$\Delta L = \frac{1}{w}\int_0^w \sqrt{\frac{Dl}{u}}dl = \frac{2}{3}\sqrt{\frac{Dw}{u}}, \tag{7}$$

and this represents the effective extension of the mixing region.

The maximum flow rate inside a wide, flat rectangular channel is

$$u = \frac{\Delta P}{8\eta}\frac{h^2}{L} \tag{8}$$

Combining equations 7 and 8 and the Stokes-Einstein equation ($D = \frac{k_B T}{6\pi\eta r}$) gives

$$\Delta L = \frac{4}{3}\sqrt{\frac{k_B T w L}{3\pi \Delta P r h^2}}. \tag{9}$$

Here $w$, $L$, and $h$ are the width, length, and height of the microchannel. Notice that eq. 9 does not depend on the properties of the solution, only parameters that did not vary in our experiments. Using the experimental values gives a $\Delta L$ of $27\,\mu\mathrm{m}$. The boundary regions at the ends of the mixing channel are relatively small compared with the length of the mixing channel itself. In our analyses, we accounted for the small effective extension of the mixing channel due to diffusive mixing at the ends by taking $L = L_{mixing} + 2 \times 27\,\mu\mathrm{m}$, where $L_{mixing}$ is the measured length of the mixing channel.

**Chemical potential gradient**

A gradient in the chemical potential of ions can drive a current. To eliminate this as a possible explanation for the current that we measured, we estimated the effect of a chemical potential gradient arising from the inhomogeneous solvent.

*Ions in the bulk liquid*

If an ion has a different solvation energy in glycerol/water than in formamide/water, there will be a chemical force acting to drive it toward a lower chemical potential and resulting in an electrical current. In particular, if $K^+$ has a lower solvation energy in glycerol than in formamide, a net current of these ions could flow toward regions of higher glycerol concentration. Similarly, if $Cl^-$ has a lower solvation energy in formamide than glycerol, a net current of these ions could flow toward regions of higher formamide concentration. Furthermore, we expect a chemically-driven current to grow in magnitude with the magnitude of the viscosity gradient, because the viscosity gradient reflects the gradient in the chemical composition of the liquid. Therefore, a chemical potential gradient could generate a current similar to the one we have measured and attributed to viscophoresis. However, such a current would scale linearly with the bulk salt concentrations. In constrast, we found that the bulk KCl salt concentration had almost no effect on the measured current, so we can rule out bulk ion transport due to chemical potential gradients as the cause of the viscophoretic current.

*Surface*

The bulk argument presented above does not rule out the possibility that chemical potential gradients give rise to currents in the electric double layers near surfaces. There can exist a gradient in the chemical potential of $K^+$ that drives it in the direction of increasing formamide content; the absence of a bulk ionic current only implies that the chemically driven motion of $K^+$ must be offset by an equivalent motion of $Cl^-$ in the same direction. In the electric double layers, there is an excess of $K^+$, so the motion of that ion will no longer be offset by $Cl^-$. We know from the absence of a bulk ionic current that $K^+$ and $Cl^-$ experience the same chemical potential differences between glycerol and formamide, and we can estimate those chemical potential differences based on KCl solubilities.

The change in free energy associated with the dissolution of KCl ($\mathrm{KCl} \longrightarrow \mathrm{K}^+ + \mathrm{Cl}^-$) in solvent $i$, $\Delta G_i$, is

$$\Delta G_i = \mu_{0,i}^{\mathrm{K}^+} + \mu_{0,i}^{\mathrm{Cl}^-} - \mu_{0,i}^{\mathrm{KCl}} + k_B T \log(C_i^{\mathrm{K}^+} C_i^{\mathrm{Cl}^-}), \tag{10}$$

where $\mu_{0,i}^x$ is the standard chemical potential of species $x$ in solvent $i$, and $C_i^{\mathrm{K}^+}$ and $C_i^{\mathrm{Cl}^-}$ are the concentrations of $K^+$ and $Cl^-$, respectively. When the concentrations of $K^+$ and

$Cl^-$ are constant and equal to each other, as they are in our experiments, the change in free energy as KCl moves from glycerol to formamide, $\Delta G_{g\to f}$, is

$$\Delta G_{g\to f} = \mu_0^{K,g} + \mu_0^{Cl,g} - \mu_0^{K,f} - \mu_0^{Cl,f}. \quad (11)$$

We can relate eq. 11 to the solubilities of KCl in glycerol and formamide. We begin by noting that at the saturation concentration, $C_{i,sat} = C_i^{\mathrm{K}^+} = C_i^{\mathrm{Cl}^-}$, dissolving additional KCl does not lower the free energy, and $\Delta G_i = 0$ in eq. 10 implies

$$\mu_{0,i}^{\mathrm{K}^+} + \mu_{0,i}^{\mathrm{Cl}^-} - \mu_{0,i}^{\mathrm{KCl}} = -k_B T \log[(C_{i,sat})^2]. \quad (12)$$

Combining eqs. 11 and 12 obtains

$$\Delta G_{g\to f} = \mu_{0,f}^{\mathrm{KCl}} - \mu_{0,g}^{\mathrm{KCl}} - 2k_B T \log\left(\frac{C_{f,sat}}{C_{g,sat}}\right). \quad (13)$$

Because KCl is a solid, its chemical potential cannot depend on the solvent. Therefore, $\mu_{0,f}^{\mathrm{KCl}} = \mu_{0,g}^{\mathrm{KCl}}$, and eq. 13 simplifies to

$$\Delta G_{g\to f} = 2k_B T \log\left(\frac{C_{g,sat}}{C_{f,sat}}\right). \quad (14)$$

The free energy change in eq. 14 occurs over the length of the mixing channel, so the effective force $F$ that it exerts on salt ions inside the mixing channel is

$$F = \frac{2k_B T}{L} \log\left(\frac{C_{g,sat}}{C_{f,sat}}\right). \quad (15)$$

If we model the viscous drag on the ions with Stokes' drag on a sphere of radius $r$, the resulting drift speed is

$$v = \frac{F}{6\pi\eta r} = \frac{k_B T}{3\pi\eta r L} \log\left(\frac{C_{g,sat}}{C_{f,sat}}\right). \quad (16)$$

The drift of ions can result in a net current where there is an imbalance in the density of positive and negative ions, namely, in the electric double layers near the channel surfaces. For a channel with $w \gg L$, we can neglect edge effects and approximate the current as $I = 2\sigma w v$, which is combined with eq. 16 to obtain

$$I = \frac{F}{6\pi\eta r} = \frac{2}{3} k_B T \frac{\sigma}{\pi\eta r} \frac{w}{L} \log\left(\frac{C_{g,sat}}{C_{f,sat}}\right). \quad (17)$$

The saturation concentrations for KCl in glycerol and formamide are $1106\,\mathrm{mM}$ and $939\,\mathrm{mM}$, respectively [1, 3]. Using pure formamide and glycerol concentrations and typical parameters from our experiment ($w = 150\,\mu\mathrm{m}$, $L = 200\,\mu\mathrm{m}$, $r = 1.25\,\text{Å}$), and the measured viscosity of an equal glycerol-formamide mixture, $\eta = 21.2\,\mathrm{mPa\,s}$, gives only $8\,\mathrm{pA}$. Therefore, we conclude that chemical forces cannot account for more than a small fraction of the currents we measured.

**Streaming current**

Streaming currents are a potential alternate explanation for the currents we have measured. However, we have found that the currents do not immediately die when the microchannel flows are turned off. This observation is not consistent with streaming current.

Further, estimates of streaming current show the effect to be far too small. A measurement of streaming current in a similar glass nanochannel gives a good estimate of the magnitude. The Dekker group found a current of less than $10\,\mathrm{pA}$ of streaming current driven by $1\,\mathrm{bar}$ of pressure in a water-filled nanochannel $4.5\,\mathrm{mm}$ long, $50\,\mu\mathrm{m}$ wide, and $100\,\mathrm{nm}$ tall. Our nanochannel is 22.5 times longer and three times wider. This results in more streaming current. It is also half as tall and has at least double the viscosity. This overall leads to an estimate of $84\,\mathrm{pA\,bar}^{-1}$. This means that even $100\,\mathrm{mbar}$ across our nanochannel could only drive $8.4\,\mathrm{pA}$. This is not enough to explain the effect we have measured.

**Bernoulli effect**

The viscosities in the microchannels are different, so the flow rates are also different. This introduces the possibility of a pressure difference across the mixing channel. Again, this effect would stop as soon as flow stops, but the current we have measured persists.

An estimate of the magnitude of this effect also shows it to be far too small. Bernoulli's principle says

$$P + \frac{\rho v^2}{2} = const \quad (18)$$

Comparing the points at either end of the nanochannel,

$$P_L + \frac{\rho_R v_L^2}{2} = P_R + \frac{\rho_R v_R^2}{2} \quad (19)$$

$$P_L - P_R = \frac{1}{2}\left(\rho_R v_R^2 - \rho_L v_L^2\right) \quad (20)$$

The maximum flow rate in a rectangular channel of width $w$, height $h$, and length $l$, where $w >> h$ is

$$u_{max} = \frac{h^2 P_a}{8\eta l}, \quad (21)$$

where $P_a$ is the pressure applied to the microchannels, and $\eta$ is the viscosity.

The pressure arising as a result of Bernoulli's principle is,

$$P_L - P_R = \frac{P_a}{128} \frac{h^4}{l^2} \left(\frac{\rho_R}{\eta_R^2} - \frac{\rho_L}{\eta_L^2}\right) \quad (22)$$

This amounts to about $5 \times 10^{-11}\,\mathrm{bar}$. Using the above estimate of $84\,\mathrm{pA\,bar^{-1}}$ gives a minuscule current of $4.2 \times 10^{-9}\,\mathrm{pA}$

---

[1] Burgess, J., *Metal ions in solution* (1978).

[2] Rehfeldt, S. and Stichlmair, J., Fluid phase equilibria **256**, 99 (2007).

[3] Seidell, A. *et al.*, *Solubilities of inorganic and organic compounds* (van Nostrand, 1952).

[4] Sokolov, I., Chemical Physics **375**, 359 (2010).

[5] Vignes, A., Industrial & Engineering Chemistry Fundamentals **5**, 189 (1966).

[6] Volpe, G. and Wehr, J., Reports on Progress in Physics **79**, 053901 (2016).
